# Supplementary material for: Design Space Exploration on Efficient and Accurate Human Pose Estimation from Sparse IMU-Sensing
Source: arXiv:2308.02397 source file (2024-02-12)
Supplement: Supplementary file 1 [file 6_appendix.tex]

\section{Virtual Sensors}

Each sensor position from \autoref{fig:basic_sensor_configuration} is internally represented through a Vertex ID on the SMPL+H mesh.
The Joint ID denotes the joint of the SMPL skeleton that directly actuates the virtual sensor.
Sensor ID 5 and 19 are inspired by the Xsens positioning but slightly displaced due to symmetry: The sensors at vertex ID 5287 and 1176 in Xsens are displaced to 4197 and 1177, respectively.

\begin{table}[!htb]
    \centering
    \caption{\textbf{Basic sensor configuration} indicating all sensors considered for the \gls{dse}. The sensors are sorted by distance from root sensor (vertex index 3021). All vertex and joint indices are related to the \gls{smpl}.}
    \begin{tabular}{c|c|c|l}
         Sensor ID & Vertex ID (\gls{smpl}) & Joint ID (\gls{smpl}) & dist \\
         \hline
         0  & 3021 & 0  & 0 \\
         1  & 3016 & 3  & 0.15647505 \\
         2  & 3496 & 9  & 0.3671748 \\
         3  & 4362 & 2  & 0.3722757 \\
         4  & 876  & 1  & 0.37316912 \\
         5  & 4197 & 14 & 0.39544925 \\
         6  & 707  & 13 & 0.3979012 \\
         7  & 1305 & 9  & 0.4103658 \\
         8  & 958  & 1  & 0.4610727 \\
         9  & 4444 & 2  & 0.46173838 \\
         10 & 5335 & 17 & 0.48945138 \\
         11 & 1874 & 16 & 0.49041077 \\
         12 & 1719 & 16 & 0.53829616 \\
         13 & 5188 & 17 & 0.53868234 \\
         14 & 4516 & 2  & 0.5407919 \\
         15 & 1032 & 1  & 0.5408928 \\
         16 & 1623 & 18 & 0.61126786 \\
         17 & 5092 & 19 & 0.61135274 \\
         18 & 4662 & 5  & 0.7051227 \\
         19 & 1177 & 4  & 0.70617384 \\
         20 & 411  & 12 & 0.72784156 \\
         21 & 5424 & 19 & 0.79017997 \\
         22 & 1961 & 18 & 0.7946686 \\
         23 & 3322 & 4  & 0.95263433 \\
         24 & 6723 & 5  & 0.9528295 \\
    \end{tabular}
    \label{tab:sensor_config}
\end{table}

\section{AMASS Dataset}

In table \autoref{tab:AMASS_data_used}, the AMASS subsets are listed that have been used by \gls{dip} and our approach. 
Due to the active development of the AMASS dataset our database is missing the CMU\_Kitchen, and MIXAMO dataset which are not included anymore.
For compensation of the data volume additional dataset are added.
These are DanceDB, DFaust\_67, EKUT, KIT, MPI\_mosh, SFU, and TCD\_handMocap.

\begin{table}[!ht]
    \centering
    \begin{tabular}{|l|l|r|l|r|}
        \hline
        \textbf{DIP} & \textbf{Ours – Matching}  & \textbf{Minutes} & \textbf{Ours - Additional} & \textbf{Minutes} \\ \hline
        ACCAD & ACCAD & 26.74 & DanceDB & 203.38 \\ \hline
        BioMotion & BioMotionLab\_NTroje & 522.69 & DFaust\_67 & 5.72 \\ \hline
        CMU & CMU & 543.49 & EKUT & 30.74 \\ \hline
        CMU\_Kitchen & ~ & no data & KIT & 661.84 \\ \hline
        Eyes & Eyes\_Japan\_Dataset & 397.04 & MPI\_mosh & 16.53 \\ \hline
        HDM05 & HDM05 & 144.54 & SFU & 15.23 \\ \hline
        HEva & HumanEva & 8.47 & TCD\_handMocap & 8.37 \\ \hline
        JointLimit & MPI\_Limits & 20.82 & ~ & ~ \\ \hline
        MIXAMO & ~ & no data & ~ & ~ \\ \hline
        SSM & SSM\_synced & 1.87 & ~ & ~ \\ \hline
        Transition & Transitions\_mocap & 15.10 & ~ & ~ \\ \hline \hline
        Total & ~ & 1680.76 & ~ & 941.81 \\ \hline
    \end{tabular}
    \caption{Comparison of AMASS sub-dataset used by \gls{dip}~\cite{Huang2018} and our equivalent. \todo{Fix table width - potentially remove}}
    \label{tab:AMASS_data_used}
\end{table}
